# Supplementary material for: Phase transformation and synchrony for a network of coupled Izhikevich neurons
Source: arXiv:2407.20055 ancillary file (2024-07-29)
Supplement: Supplementary file 1 [file izhikevich_phase_supplemental_material.pdf]

# Phase transformation and synchrony for a network of coupled Izhikevich neurons

Supplemental material

July 29, 2024

## Mean-field derivation

We consider a network of $N$ globally coupled conductance-based Izhikevich neurons,

$$C_m \frac{\mathrm{d}v_j}{\mathrm{d}t} = k(v_j - v_\theta)(v_j - v_r) - u_j + \eta_j + s(v_{\text{syn}} - v_j), \tag{1}$$

$$\frac{\mathrm{d}u_j}{\mathrm{d}t} = a(b(v_j - v_r) - u_j), \tag{2}$$

where $j = 1, \ldots, N$, $v_j(t) \to v_{reset}$ and $u_j(t) \to u_j(t) + u_{jump}$ when $v_j(t) > v_{th}$. As outlined in the manuscript, we consider first order synaptic coupling,

$$\tau_s \frac{\mathrm{d}s}{\mathrm{d}t} = -s + \frac{\kappa}{N} \sum_{l=1}^{N} \sum_{m} \delta(t - t_l^m), \tag{3}$$

where $t_l^m$ is the $m$th spike time of the $l$th neuron and $\kappa$ is the synaptic coupling strength.

Using the phase transformation

$$v_{izh}(t) = \frac{\omega}{2k} \tan\left(\frac{1}{2}\omega t + d\right) + \frac{v_\theta + v_r}{2}, \tag{4}$$

we arrive at the equations given in the manuscript

$$C_m \frac{\mathrm{d}\theta_j}{\mathrm{d}t} = 1 - \cos\theta_j + k\left(1 + \cos\theta_j\right)\left[-\frac{k}{4}(v_\theta - v_r)^2 - u_j + \eta_j + s\left(v_{syn} + \frac{v_\theta + v_r}{2}\right)\right] - s\sin\theta_j, \tag{5}$$

$$\frac{\mathrm{d}u_j}{\mathrm{d}t} = a\left[b\left(\frac{1}{k}\tan\frac{\theta_j}{2} + \frac{v_\theta + v_r}{2}\right) - u_j\right], \tag{6}$$

for $j = 1, \ldots, N$, and $u_j(t) \to u_j(t) + u_{jump}$ when $\theta_j(t)$ increases through $\pi$.

The Ott-Antonsen ansatz [2] can be applied to networks of phase oscillators whose individual

dynamics take the following form

$$\frac{\mathrm{d}\theta}{\mathrm{d}t} = f\mathrm{e}^{i\theta} + h + \bar{f}\mathrm{e}^{i\theta}. \tag{7}$$

The reduced model takes the form

$$\frac{\mathrm{d}\alpha}{\mathrm{d}t} = -i\left[\alpha^2 f + \alpha h + \hat{f}\right], \tag{8}$$

where $\alpha(\eta, t)$ is related to the Kuramoto order parameter $Z(t)$ as follows

$$\bar{Z}(t) = \int_{-\infty}^{\infty} \mathrm{d}\eta \mathcal{L}(\eta)\alpha(\eta, t) = \alpha(\eta_0 + i\Delta, t), \tag{9}$$

where $\mathcal{L}(\eta)$ is a Lorentzian distribution, with centre $\eta_0$ and full width at half maximum $\Delta$, from which the background drives $\eta_j$ are drawn.

To write (5) in the form given by (7), we let

$$f = \frac{1}{2C_m}(-1 + \Pi + iks), \qquad h = \frac{1}{C_m}(1 + \Pi),$$

where $\Pi = k\left(-\frac{k}{4}(v_\theta - v_r)^2 - u + \eta + s\left(v_{syn} + \frac{v_\theta + v_r}{2}\right)\right)$. Subbing this into (8) and evaluating at $\eta = \eta_0 + i\Delta$, allows us define the dynamics of the Kuramoto order parameter

$$C_m\frac{\mathrm{d}Z}{\mathrm{d}t} = -i\frac{(Z-1)^2}{2} + k\frac{(Z+1)^2}{2}\left(i\left[-\frac{k}{4}(v_\theta - v_r)^2 - u + \eta_0 + s\left(v_{syn} + \frac{v_\theta + v_r}{2}\right)\right] - \Delta\right) - s\frac{Z^2 - 1}{2}, \tag{10}$$

where $u = \frac{1}{N}\sum_j u_j$,

$$\frac{\mathrm{d}u}{\mathrm{d}t} = a\left(b(V(Z) - v_r) - u\right) + u_{\text{jump}} f(Z), \tag{11}$$

$$\tau_s\frac{\mathrm{d}s}{\mathrm{d}t} = -s + \kappa f(Z). \tag{12}$$

The functions $f(Z)$ and $V(Z)$ are given as

$$f(Z) = \frac{1}{\pi C_m}\frac{1 - |Z|^2}{1 + Z + \bar{Z} + |Z|^2},$$

$$V(Z) = \frac{1}{k}\frac{\mathrm{Im}(Z)}{1 + Z + \bar{Z} + |Z|^2} + \frac{v_\theta + v_r}{2},$$

## Mean-field validation for fast spiking cells

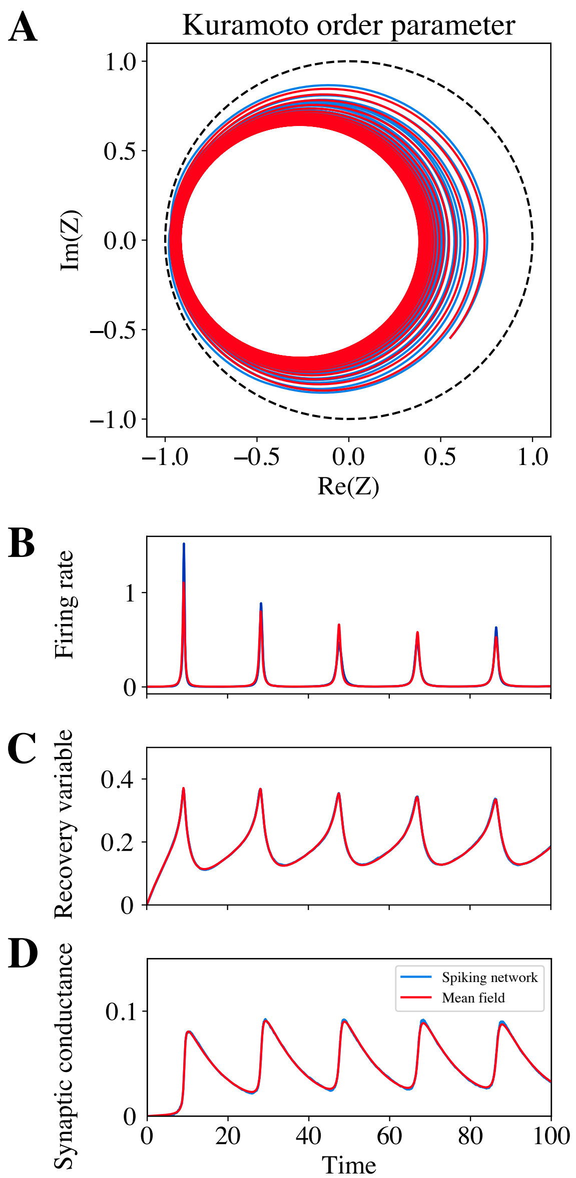


Figure S1: **Mean-field validation:** Comparison of the Kuramoto order parameter (A), firing rate (B), recovery variable (C) and synaptic conductance (D) for the reduced mean field model (red and a simulation of a network of 200 fast spiking Izhikevich neurons (blue).

## Mean-field equations for two population model

For the network model, the system becomes 10-dimensional

$$\begin{aligned}
C_m^E \frac{\mathrm{d}Z_E}{\mathrm{d}t} &= -i\frac{(Z_E-1)^2}{2} + k_E\frac{(Z_E+1)^2}{2}\left(i\left[-\frac{k_E}{4}(v_\theta^E - v_r^E)^2 - u_E + \eta_0^E + s_{EE}v_{syn}^E + s_{IE}v_{syn}^I \right.\right. \\
&\quad \left.\left. +\ (s_{EE}+s_{IE})\left(\frac{v_\theta^E + v_r^E}{2}\right)\right] - \Delta_E\right) - (s_{EE}+s_{IE})\frac{Z_E^2-1}{2}, \qquad (13)\\
C_m^I \frac{\mathrm{d}Z_I}{\mathrm{d}t} &= -i\frac{(Z_I-1)^2}{2} + k_I\frac{(Z_I+1)^2}{2}\left(i\left[-\frac{k_I}{4}(v_\theta^I - v_r^I)^2 - u_I + \eta_0^I + s_{EI}v_{syn}^E + s_{II}v_{syn}^I \right.\right. \\
&\quad \left.\left. +\ (s_{EI}+s_{II})\left(\frac{v_\theta^I + v_r^I}{2}\right)\right] - \Delta_I\right) - (s_{EI}+s_{II})\frac{Z_I^2-1}{2}, \qquad (14)\\
\frac{\mathrm{d}u_E}{\mathrm{d}t} &= a_E\left(b_E(V(Z_E) - v_r^E) - u_E\right) + u_{\text{jump}}^E f(Z_E), \qquad (15)\\
\frac{\mathrm{d}u_I}{\mathrm{d}t} &= a_I\left(b_I(V(Z_I) - v_r^I) - u_I\right) + u_{\text{jump}}^I f(Z_I), \qquad (16)\\
\tau_{s_E}\frac{\mathrm{d}s_{EE}}{\mathrm{d}t} &= -s_{EE} + \kappa_{EE} f(Z_E), \qquad (17)\\
\tau_{s_I}\frac{\mathrm{d}s_{IE}}{\mathrm{d}t} &= -s_{IE} + \kappa_{IE} f(Z_I), \qquad (18)\\
\tau_{s_E}\frac{\mathrm{d}s_{EI}}{\mathrm{d}t} &= -s_{EI} + \kappa_{EI} f(Z_E), \qquad (19)\\
\tau_{s_I}\frac{\mathrm{d}s_{II}}{\mathrm{d}t} &= -s_{II} + \kappa_{II} f(Z_I). \qquad (20)
\end{aligned}$$

The functions $f(Z)$ and $V(Z)$ are given as

$$\begin{aligned}
f(Z) &= \frac{1}{\pi C_m}\frac{1-|Z|^2}{1+Z+\bar{Z}+|Z|^2}, \\
V(Z) &= \frac{1}{k}\frac{\mathrm{Im}(Z)}{1+Z+\bar{Z}+|Z|^2} + \frac{v_\theta + v_r}{2}.
\end{aligned}$$

## Parameter values

**Regular spike neurons**

| | |
|---|---|
| $C_m$ | 100 |
| $k$ | 0.7 |
| $v_\theta$ | -40 |
| $v_r$ | -60 |
| $v_{syn}$ | 0 |
| $\kappa$ | 15 |
| $\tau_S$ | 3 |
| $v_{th}$ | 14235.7 |
| $v_{reset}$ | -14335.7 |
| $a$ | 0.03 |
| $b$ | -2 |
| $u_{jump}$ | 10 (weak)<br>100 (strong ) |

**Fast spike neurons**

| | |
|---|---|
| $C_m$ | 20 |
| $k$ | 1 |
| $v_\theta$ | -40 |
| $v_r$ | -55 |
| $v_{syn}$ | -65 |
| $\kappa$ | 15 |
| $\tau_S$ | 10 |
| $v_{th}$ | 9952.5 |
| $v_{reset}$ | -10047.5 |
| $a$ | 0.2 |
| $b$ | 0.025 |
| $u_{jump}$ | 0 |

**Coupling strengths for RS-FS network**

| | |
|---|---|
| $\kappa_{EE}$ | 10 |
| $\kappa_{IE}$ | 4 |
| $\kappa_{EI}$ | 10 |
| $\kappa_{II}$ | 4 |

The threshold $v_{th}$ and reset $v_{reset}$ are calculated as $\frac{1}{k}\left(\pm 10000 + \frac{v_r + v_\theta}{2}\right)$, respectively. This produces symmetric spikes and ensures maximal accuracy of the mean-field reduction. See [1] for how to deal with asymmetric spikes.

## References


[1] Ernest Montbrió and Diego Pazó. Exact mean-field theory explains the dual role of electrical synapses in collective synchronization. *Phys. Rev. Lett.*, 125:248101, Dec 2020. doi: 10.1103/PhysRevLett.125.248101.

[2] Edward Ott and Thomas M Antonsen. Low dimensional behavior of large systems of globally coupled oscillators. *Chaos: An Interdisciplinary Journal of Nonlinear Science*, 18(3), 2008.
